# Supplementary material for: Composable Energy Policies for Reactive Motion Generation and Reinforcement Learning
Source: arXiv:2105.04962 source file (2021-05-11)
Supplement: Supplementary file 1 [file old_appendix.tex]

\label{sec:optimality}
In the following section, we want to highlight the connections between \gls{cep} and Max-Ent optimal control in order to evaluate the optimality guarantees of composing energies in a multi-objective optimal control problem.


\begin{figure}[ht]
	\caption{Graphical model for the Optimal Control problem. $\vs_t$ denoted the state, $\va_t$ denotes the action and $o_t$ is an additional variable representing the optimality of the state and action for a given reward.}
	\begin{center}
		\input{img/models/tikz_test}
	\end{center}
	\label{fig:factor_graph_0}
\end{figure}


We frame optimal control as Bayesian inference problem~\cite{rawlik2012stochastic,levine2018reinforcement} over the sequence of actions $\va_{0:T}$. The optimal control problem is visualized as a factor graph in Fig.~\ref{fig:factor_graph_0}. The problem is formulated introducing an auxiliary variable $o_{0:T}$ that represents the optimality of $\vs_t$ and $\va_t$ under a certain reward function, $p(o_{t}|\vs_t, \va_t) \propto \exp(r(\vs_t,\va_t))$. Given a certain prior distribution $q(\va|\vs_0)$ and given $\vs_0$ is known, the inference problem is
\begin{align}
	\label{eq:control_as_inference}
	p(A_{0}^{T} | \vs_0, O_{0}^{T} ) = \frac{p(O_{0}^{T}|A_{0}^{T},\vs_0) q(A_{0}^{T}|\vs_0)}{p(O_{0}^{T}|\vs_0)}
\end{align}
with
\begin{align}
	p(O_{0}^{T}|A_{0}^{T},\vs_0) = \int_{\vs_{1:T}} p(O_{0}^{T}|S_{0}^{T},A_{0}^{T})p(S_{1}^{T}|A_{0}^{T},\vs_0)d S_{1}^{T}
\end{align}
where $A_{0}^{T}:\{\va_0,\dots, \va_T\}$, $O_{0}^{T}:\{o_0,\dots, o_T\}$ and  $S_{0}^{T}:\{\vs_0,\dots, \vs_T\}$.
The are two main directions to solve the posterior in \eqref{eq:control_as_inference}. First, methods that frame the problem as an \gls{hmm} and solve it in a Expectation-Maximization approach. Second, methods that computes the posterior in the trajectory level $A_{0}^{T}$. The first, are computationally demanding as they require several forward and backward message passing to compute the posterior. The second, needs to solve the problem in the trajectory level and thus the variables dimension grows linearly with the trajectory length, $T$.

Reactive motion generation instead, solves a one-step ahead problem. The solutions in reactive motion generation are local rather than global and thus, they are computationally more efficient. 

We frame reactive motion generation as a one-step control as inference problem
\begin{align}
	p( \va_{0} | \vs_0, O_{0}^{T} ) = \frac{p(O_{0}^{T}|\va_{0},\vs_0)q(\va_{0}|\vs_0)}{p(O_{0}^{T}|\vs_0)}
\end{align}
with
\begin{align}
	&p(O_{0}^{T}|\va_0,\vs_0) = \nonumber \\
	&\int_{S_{1:T}}\int_{A_{1:T}} p(O_{0}^{T}|S_{0}^{T},A_{0}^{T})p(S_{1}^{T}|\va_0,\vs_0) \pi(A_{1}^{T}|S_{1}^{T})d S_{1}^{T} d A_{1}^{T}.
	\label{eq:adapted_op}
\end{align}
In contrast with the classical stochastic optimal control problem that finds the posterior for the whole trajectory $A_{0}^{T}$, in one-step ahead control as inference problem, we aim to find the posterior for only the instant next control action, $\va_0$. Computing the posterior only for $\va_0$ requires the likelihood to be defined as the marginal of not only the state trajectory $S_{1}^{T}$, but also the action trajectory $A_{1}^{T}$. The graphical model for one-step ahead control as inference is presented in Fig.~\ref{fig:one_step_optimal}.
\begin{figure}[ht]
	\caption{Graphical model for one-step ahead optimal control problem. In this approach, the actions $A_{1}^{T}$ are dependant on $S_{1}^{T}$ given a policy $\pi$.}
	\begin{center}
		\input{img/models/adapted_fact_graph}
	\end{center}
	\label{fig:one_step_optimal}
\end{figure}
In one-step ahead control as inference, we introduce an additional distribution $\pi$ that provides us the probability of $A_{1}^{T}$ given $S_1^T$. This additional policy $\pi$ is interpret as the policy the agent will apply in the future. In this context, given we know the policy the agent will apply in the future, we are looking for the instant action the maximized the cumulative reward in the long horizon trajectory. \eqref{eq:adapted_op} can be rewritten as the expectation over $p(O_{0}^{T}|S_{0}^{T},A_{0}^{T})$
\begin{align}
	\E_{S_{0}^{T},A_{0}^{T}\sim p^{\pi}(S_{0}^{T},A_{0}^{T}|\vs_0,\va_0)}\left[  p(O_{0}^{T}|S_{0}^{T},A_{0}^{T}) \right] \propto \nonumber \\
	\E_{S_{0}^{T},A_{0}^{T}\sim p^{\pi}(S_{0}^{T},A_{0}^{T}|\vs_0,\va_0)} \left[ \exp (\sum_{t=0}^{T} r(\vs_t, \va_t))\right]= \nonumber \\
	\exp(Q_{r}^{\pi}(\vs_0, \va_0))
\end{align}
From what follows, the likelihood for out inference problem is proportional to the $\exp(Q)$ defined over a certain policy $\pi$. Given a $Q$ function is given, the posterior for our inference problem is given by
\begin{align}
	p(\va_0|\vs_0, O_0^T) \propto 	\exp(Q_{r}^{\pi}(\vs_0, \va_0))q(\va_{0}|\vs_0).
\end{align}
In practise, we apply Stochastic search over $\exp(Q_{r}^{\pi}(\vs_0, \va_0))$ by iteratively applying approximate inference over $p(\va_0|\vs_0, O_0^T)$~(Alg. \ref{alg:cep}).

The provided $Q$ function depends on $\pi$ and then, the quality of our reactive motion generator to solve a long horizon optimal control problem directly depends on the quality of $\pi$. In the optimal case, for $Q^*$, reactive motion generator is able to find the optimal trajectory, even if the optimization is done locally.


\subsection{Product-Of-Experts}

We consider the problem of solving a multi-objective task by the combination of a set of modular policies $\pi_1(\va|\vs),\dots,\pi_K(\va|\vs)$. Each policy might have a different source (behavioural cloning, reinforcement learning, heuristics, optimal control) and it is assumed to solve a specific goal.

One of the most popular approaches for combining policies is the Mixture of Experts
\begin{align*}
    \pi(\va|\vs) = \sum_{k=1}^{K} \omega_k \pi_k(\va|\vs),\,  \sum_{k=1}^{K} \omega_k = 1
\end{align*}
In this approach, on each instant, a single component is activated. For sampling an action from this policy, first a skill is chosen from a categorical distribution parameterized by the weights $\omega_i$ and then, an action is sampled from the chosen component $\pi_k(\va|\vs)$.

In our work, we want the selected policy to satisfy multiple objectives at the same time. Mixture of Experts will select a unique policy per time and so, it could satisfy a unique goal. Contrarily, we propose instead to frame our policy  as a Product-of-Experts~\cite{MCPPeng19, paraschos2013probabilistic, haarnoja2018composable, tasse2020boolean}
\begin{align}
    \pi(\va | \vs) = \prod_{k=1}^{K} \pi_k(\va|\vs)^{\beta_k} \,,  \beta_k>0
    \label{eq:composed_energies}
\end{align}
were $\beta_k$ is a inverse temperature parameter. The temperature parameter will directly influence the entropy of the policy. For $\beta >1$, the entropy will shrink and the influence of the component over the composed policy increase. For $\beta < 1$, the entropy of the component will increase and the influence in the overall policy will be reduced. In the boundaries, $ \lim_{\beta \to 0} \pi(\va|\vs)^{\beta} = \gU(\va|\vs)$, will make our policy to be a uniform distribution and $\lim_{\beta \to \infty} \pi(\va|\vs)^{\beta} = \delta(\va-\argmax_\va \pi(\va|\vs)) $, it will converge to a delta distribution centered in the maximum.

Given the influence of the entropy in the overall composition, we are interested in high entropy policies. High entropy policies consider a big set of possible good actions to satisfy their objective. Thus, in the composition of several policies, high entropy policies will easily find a common interest regions in the action space. We add additional insights in the optimality of the policy composition in Appendix~\ref{sec:optimality}.
